# Supplementary material for: Lingering Dynamics in Microvascular Blood Flow
Source: arXiv:2102.12929 source file (2021-02-25)
Supplement: Supplementary file 1 [file SI.pdf]

# Supplementary information to “Lingering dynamics in microvascular blood flow”

A. Kihm, S. Quint, M. W. Laschke, M. D. Menger,
T. John, L. Kaestner, and C. Wagner

This supplementary material is structured as follows: In section S1, an overview of all geometries found in investigated hamster models and the binarized mask of the bifurcating vessel system is shown as well as the probability densities of the corresponding void durations. We emphasize that, although the total recorded dataset comprises more geometries, the shown ones are the only scenarios suitable for application of a single particle tracking due to the image quality. Section S2 is the caption of the corresponding movie being provided as a separate video file. Section S3 is the movie caption of a video illustrating the integrated intensity signal over time. In section S4 the movie caption is given for the video file that illustrates the lingering algorithm for two tracked RBCs in the microvasculature. Section S5 shows the deformation behavior of RBCs approaching an apex. All datasets and algorithms are provided upon request upon the author.

## S1 Additional lingering geometries

### S1.1 Geometry 1

The presented geometry in Fig. 1 consists of one feeding vessel (M) and two daughter vessels, with vessel (1) being the only one in the focal plane and thus the developed particle tracking algorithm is applicable. As the lingering frequency, $n_{\text{linger}}$, we define the fraction of voids associated with a lingering event and the total number of voids detected in the respective branch. For the given geometry, we find $n_{1,\text{linger}} = 0.13$. Similarly to the technique in the main article we find for the probabilities of void durations less or equal than half the mean passage time of RBCs, $P_1\left(\tau_{\text{void}} < 0.5\,\tau_{\text{RBC}}\right) = 0.44$. By only considering such voids associated with lingering scenarios, we find for the corresponding probabilities $\tilde{P}_1\left(\tau_{\text{void}} < 0.5\,\tau_{\text{RBC}}\right) = 0.02$. This reflects the observations from the geometry in the main article, where suppression of short void durations due to lingering takes place as well. However, in the case of non-lingering events, larger voids are detected as can be deducted from the tails of the probability density functions. One contribution to these long void durations is the heterogeneous distribution of RBCs in the microvascular system, leading to highly irregular spaced distances between RBCs. The diameter of the vessel is measured as $d_1 = 2.9\,\mu$m at the position of intensity measurements. Due to experimental restrictions, neither the flowrate in the mother vessel can be obtained nor the flowrate in the second draining vessel, and thus, we cannot provide a normalized flowrate of vessel (1).

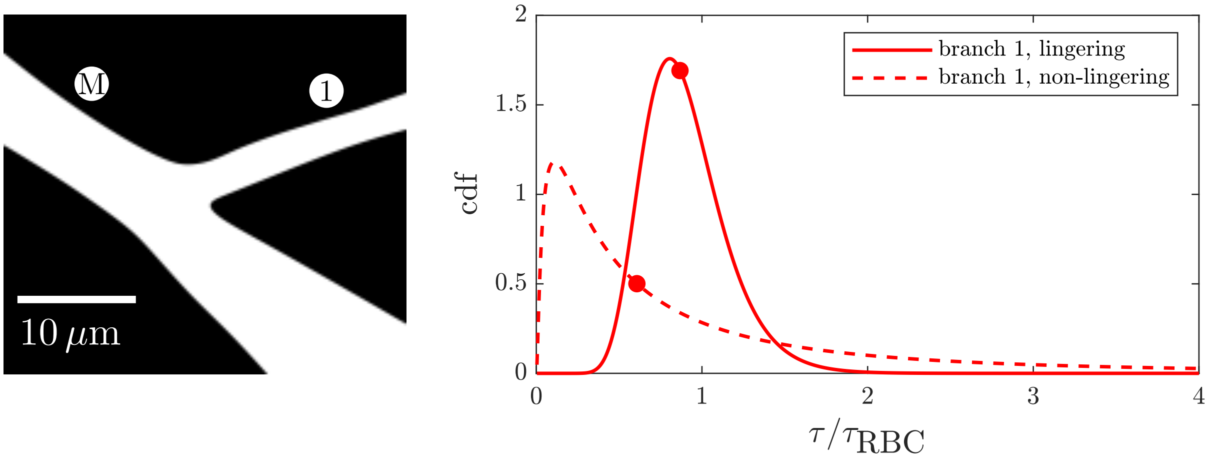


Figure 1: (left) Binary mask (evaluated manually), according to the geometry in vivo. The flow is coming from the mother vessel (M) and exits in the two daughter branches. (right) Normalized void durations associated with non-lingering events in vessel (1) (dashed line) and for lingering events (solid line). In both cases, the normalization has been obtained by the mean of all passing RBCs in the respective branch. This normalization corresponds to normalization by the flowrate. Respective median values are marked by filled circles.

## S1.2 Geometry 2

Analogously to the analysis conducted in the previous geometry we obtain a lingering frequency of $n_{1,\text{linger}} = 0.83$ whereas the second daughter vessel again is not suitable for analysis in Fig. 2. The calculated probabilities yield $P_1\left(\tau_{\text{void}} < 0.5\,\tau_{\text{RBC}}\right) = 0.33$ and $\tilde{P}_1\left(\tau_{\text{void}} < 0.5\,\tau_{\text{RBC}}\right) = 0.00$, resp. One can see out of the given void durations for both the lingering and the non-lingering case that short void durations are suppressed in the case of lingering due to redistribution of consecutive RBCs and a spatial distancing between consecutive RBCs. The measured diameter of the vessel is $d_1 = 2.8\,\mu\text{m}$, evaluated at the position of intensity measurements. As in the previous case, due to experimental restrictions flowrates are not provided.

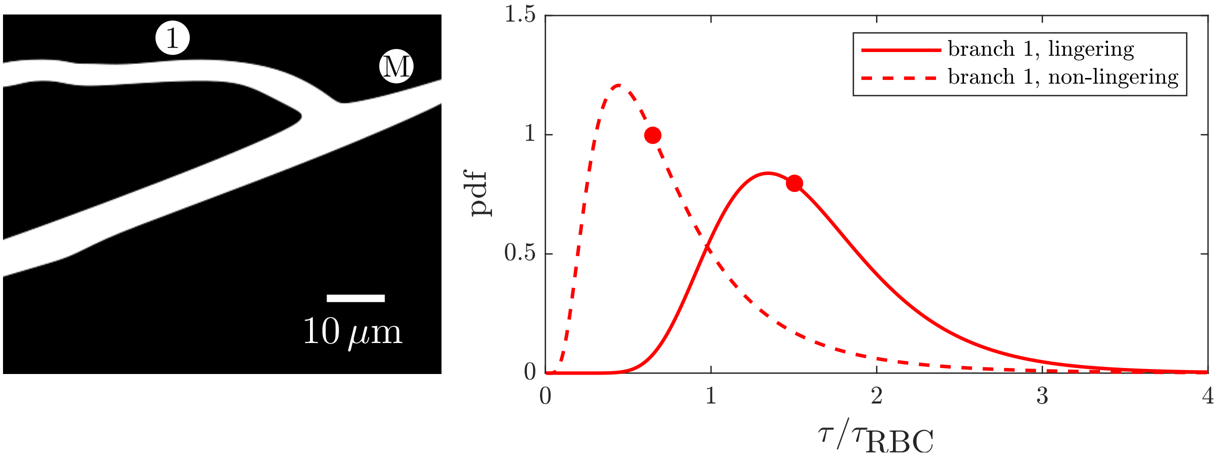


Figure 2: (left) Binary mask (evaluated manually), according to the geometry in vivo. The flow is coming from mother vessel (M) and exits in the two daughter branches. (right) Probability densities of normalized void durations associated to non-lingering events in vessel (1) (dashed line) and for lingering events (solid line). In both cases, the normalization has been obtained by the mean of all passing RBCs in the respective branch. This normalization corresponds to a normalization by the flowrate. We stress that, in the second daughter vessel, RBCs do not travel in a file but rather in a very dense suspension, not allowing for any further analysis on lingering. Respective median values are marked by filled circles.

### S1.3 Geometry 3

For the geometry depicted in Fig. 3 we calculate the lingering frequencies as $n_{i,\mathrm{linger}} = \{0.07, 0.20\}$, with $i \in \{1, 2\}$ referring to the vessel identifier. The calculated probabilities yield $P_i\,(\tau_{\mathrm{void}} < 0.5\,\tau_{\mathrm{RBC}}) = \{0.51, 0.22\}$ and $\tilde{P}_i\,(\tau_{\mathrm{void}} < 0.5\,\tau_{\mathrm{RBC}}) = \{0.06, 0.03\}$, resp. Also, the median void duration is increased in the case of lingering events. The vessel diameters yield $d_i = \{4.1, 3.5\}\,\mu$m, with corresponding normalized flowrates $q_i = Q_i/Q_{\mathrm{M}} = \{0.73, 0.27\}$.

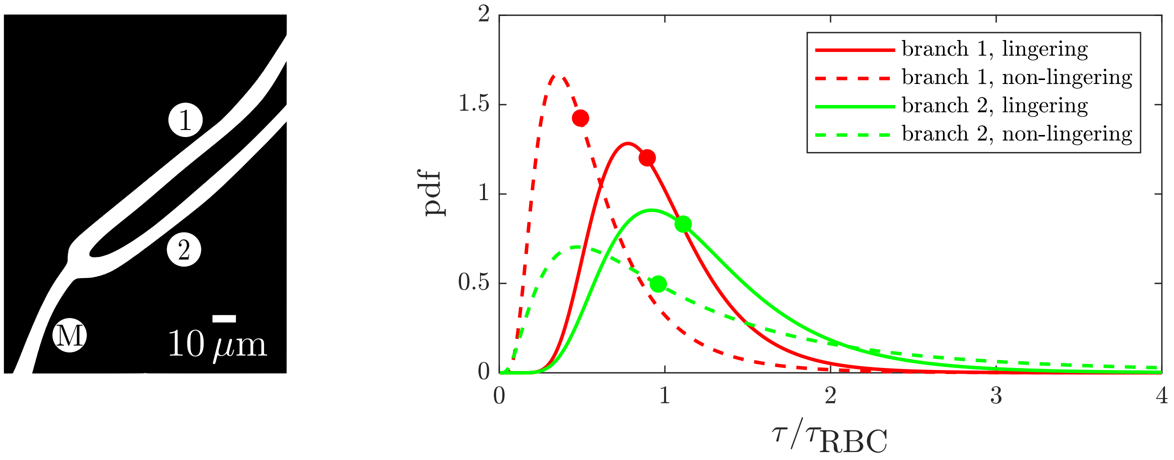


Figure 3: (left) Binary mask (evaluated manually), mimicking the geometry in vivo. The flow is coming from the lower left corner (M) and exits in the two daughter branches as denoted in the sketch. (right) Probability densities of normalized void durations associated to non-lingering events in vessels (1) and (2) (dashed lines) and for lingering events (solid line). In both cases, the normalization has been obtained by the mean of all passing RBCs in the respective branch. Respective median values are marked by filled circles.

### S1.4 Geometry 4

The obtained probabilities of void durations $\tau$ to be $\tau_{\text{void}} < 0.5\,\tau_{\text{RBC}}$ is given by $P_i\,(\tau_{\text{void}} < 0.5\,\tau_{\text{RBC}}) = \{0.45, 0.59\}$ in the case of non-lingering events and $\tilde{P}_i\,(\tau_{\text{void}} < 0.5\,\tau_{\text{RBC}}) = \{0.37, 0.34\}$ in the case of lingering events, with $i \in \{1,2\}$ referring to the vessel identifier as depicted in Fig. 4. For the lingering frequencies we find $n_{i,\text{linger}} = \{0.69, 0.42\}$, with the corresponding measured vessel diameters $d_i = \{3.1, 3.6\}\,\mu$m at the position of the signal evaluation. Corresponding average flowrates are determined as $q_i = Q_i/Q_{\text{M}} = \{0.39, 0.61\}$.

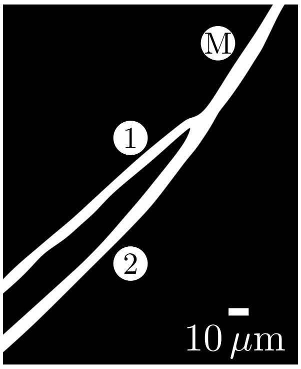


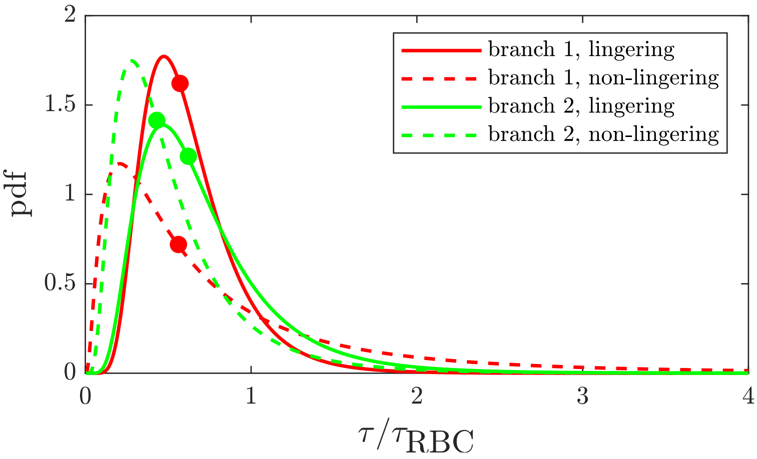


Figure 4: (left) Binary mask (evaluated manually), created according to the geometry in vivo. The flow is coming from the upper right corner (M) and exits in the two daughter branches (1) and (2), resp. as denoted in the scheme. Respective median values are marked by filled circles.

### S1.5 Geometry 5

The obtained probabilities of void durations $\tau$ to be $\tau_{\text{void}} < 0.5\,\tau_{\text{RBC}}$ is given by $P_i\,(\tau_{\text{void}} < 0.5\,\tau_{\text{RBC}}) = \{0.08, 0.01\}$ in the case of non-lingering events and $\tilde{P}_i\,(\tau_{\text{void}} < 0.5\,\tau_{\text{RBC}}) = \{0.00, 0.00\}$ in the case of lingering events, with $i \in \{1,2\}$ referring to the vessel identifier as depicted in Fig. 5. For the lingering frequencies we find $n_{i,\text{linger}} = \{0.18, 0.06\}$, with the corresponding measured vessel diameters $d_i = \{3.9, 4.2\}\,\mu$m at the position of the signal evaluation. The mean flowrates yield $q_i = Q_i/Q_{\text{M}} = \{0.31, 0.69\}$

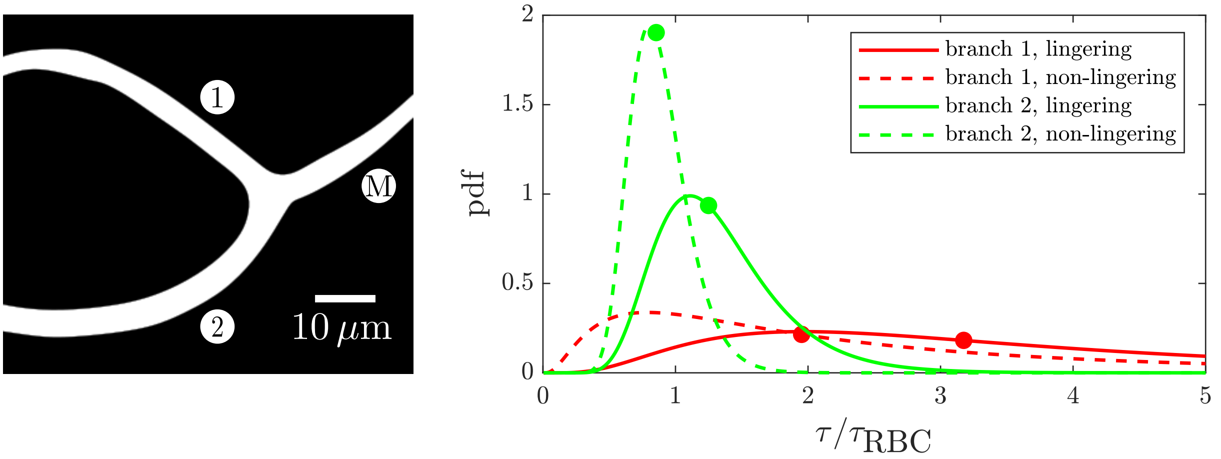


Figure 5: (left) Binary mask (evaluated manually), created according to the geometry in vivo. The flow is coming from the upper right vessel (M) and exits in the two daughter branches (1) and (2), resp. as denoted in the scheme. Respective median values are marked by filled circles.

## S1.6 Geometry 6

For the geometry depicted in Fig. 6 we calculate the lingering frequencies as $n_{i,\mathrm{linger}} = \{0.39, 0.22\}$, with $i \in \{1, 2\}$ referring to the vessel identifier. The calculated probabilities yield $P_i\,(\tau_{\mathrm{void}} < 0.5\,\tau_{\mathrm{RBC}}) = \{0.21, 0.41\}$ and $\tilde{P}_i\,(\tau_{\mathrm{void}} < 0.5\,\tau_{\mathrm{RBC}}) = \{0.09, 0.18\}$, resp. Also, the median void duration is increased in the case of lingering events. Vessel diameters yield $d_i = \{2.9, 3.3\}\,\mu$m and we find for the normalized mean flowrates $q_i = Q_i/Q_{\mathrm{M}} = \{0.31, 0.69\}$.

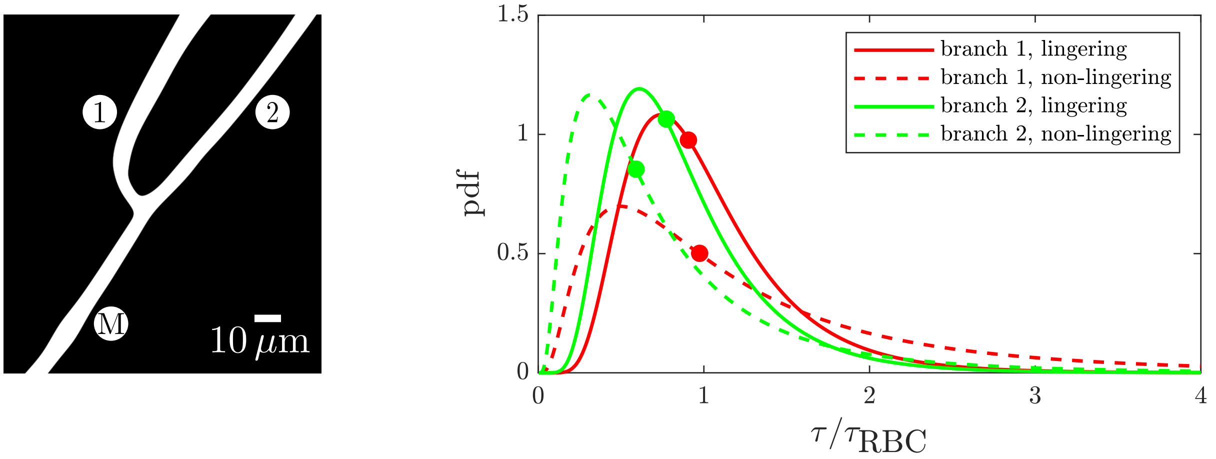


Figure 6: (left) Binary mask (evaluated manually), created according to the geometry in vivo. The flow is coming from the lower left corner (M) and exits in the two daughter branches (1) and (2), resp. as denoted in the scheme. Respective median values are marked by filled circles.

## S1.7 Geometry 7

For the geometry depicted in Fig. 7 we calculate the lingering frequencies as $n_{i,\mathrm{linger}} = \{0.28, 0.36\}$, with $i \in \{1, 2\}$ referring to the vessel identifier. The calculated probabilities yield $P_i\,(\tau_{\mathrm{void}} < 0.5\,\tau_{\mathrm{RBC}}) = \{0.55, 0.55\}$ and $\tilde{P}_i\,(\tau_{\mathrm{void}} < 0.5\,\tau_{\mathrm{RBC}}) = \{0.32, 0.49\}$, resp. to find void durations less than half the mean passage time of RBCs. Also, the median void duration is increased in the case of lingering events. We again find the vessel with the smaller diameter

obeying a higher lingering frequency compared to the bigger vessel, since the vessel diameters yield $d_i = \{3.1, 2.9\}$ $\mu$m, with average normalized flowrates $q_i = Q_i/Q_\mathrm{M} = \{0.59, 0.41\}$.

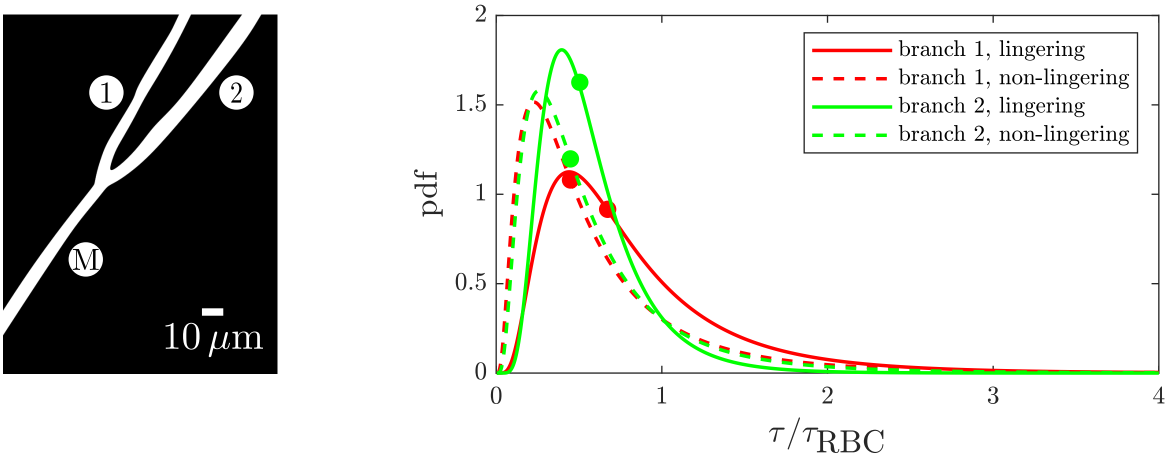


Figure 7: (left) Binary mask (evaluated manually), created according to the geometry in vivo. The flow is coming from the lower left corner (M) and exits in the two daughter branches (1) and (2), resp. as denoted in the scheme. Respective median values are marked by filled circles.

## S1.8 Geometry 8

For the geometry depicted in Fig. 8 we calculate the lingering frequencies as $n_{i,\mathrm{linger}} = \{0.74, 0.72\}$, with $i \in \{1, 2\}$ referring to the vessel identifier. The calculated probabilities yield $P_i\left(\tau_\mathrm{void} < 0.5\,\tau_\mathrm{RBC}\right) = \{0.34, 0.34\}$ and $\tilde{P}_i\left(\tau_\mathrm{void} < 0.5\,\tau_\mathrm{RBC}\right) = \{0.46, 0.37\}$, resp. to find void durations less than half the mean passage time of RBCs. Although vessel (2) shows similar behavior to the previous results of various geometries, vessel (1) shows opposite behavior. There, the median of void durations not associated to lingering events is increased compared to the lingering case. By further inspection, RBCs travel highly heterogeneous in vessel (1), leading to long RBC depleted zones and thus causing long tails in the probability density distribution of voids. Diameters of both vessels have been determined to $d_i = \{3.3, 2.9\}$ $\mu$m and mean flowrates are determined as $q_i = Q_i/Q_\mathrm{M} = \{0.43, 0.57\}$.

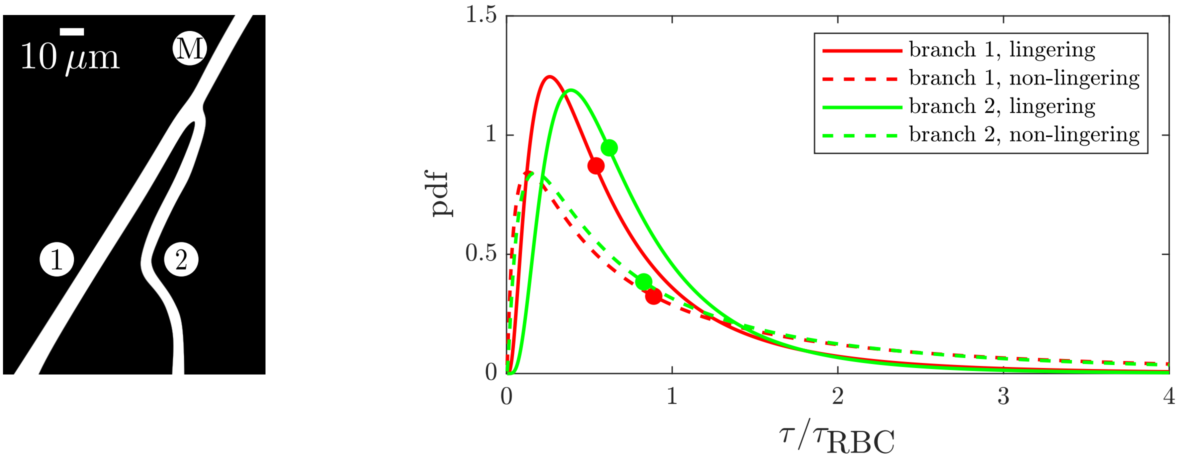


Figure 8: (left) Binary mask (evaluated manually), created according to the geometry in vivo. The flow is coming from the upper right corner (M) and exits in the two daughter branches (1) and (2), resp. as denoted in the scheme. Respective median values are marked by filled circles.

## S1.9 Geometry 9

Of all analyzed geometries, the one depicted in 9 is the only one where no lingering events occur (we recall that a lingering event takes place according to the main article, if the velocities of RBCs yield $v_{\mathrm{RBC}} < 30\,\mu\mathrm{m/s}$ in a circular region around the bifurcation apex. Thus, $n_{i,\mathrm{linger}} = \{0.00, 0.00\}$, $i \in \{1, 2\}$ referring to the vessel identifier. The diameters of the vessels are $d_i = \{2.2, 2.9\}\,\mu\mathrm{m}$ at the position of the brightness signal evaluation.

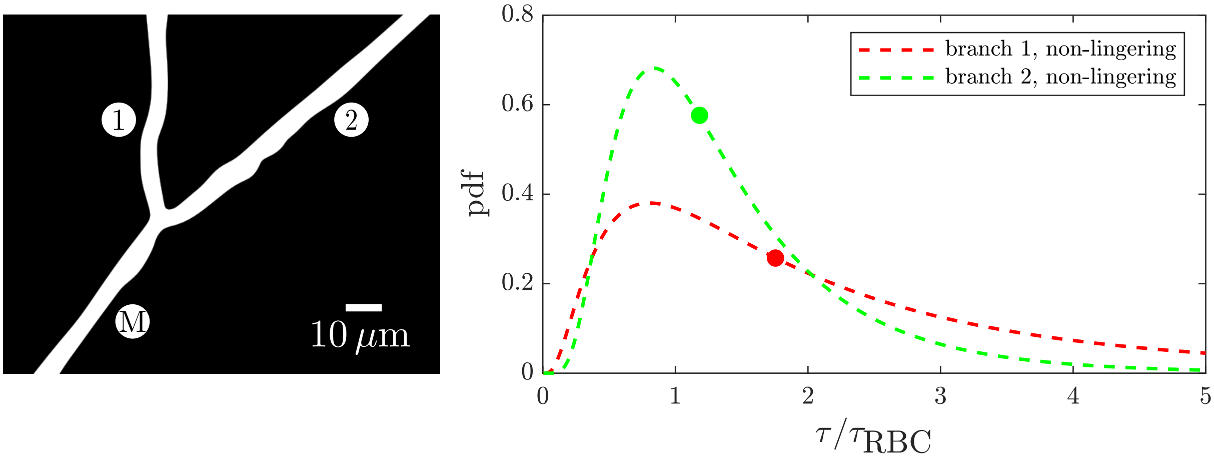


Figure 9: (left) Binary mask (evaluated manually), created according to the geometry in vivo. The flow is coming from the lower left corner (M) and exits in the two daughter branches (1) and (2), resp. as denoted in the scheme. Respective median values are marked by filled circles.

## S1.10 Geometry 10

For the geometry depicted in Fig. 10 we calculate the lingering frequencies as $n_{i,\mathrm{linger}} = \{0.79, 0.80\}$, with $i \in \{1, 2\}$ referring to the vessel identifier. The calculated probabilities yield $P_i\,(\tau_{\mathrm{void}} < 0.5\,\tau_{\mathrm{RBC}}) = \{0.29, 0.00\}$ and $\tilde{P}_i\,(\tau_{\mathrm{void}} < 0.5\,\tau_{\mathrm{RBC}}) = \{0.44, 0.44\}$, resp. to find void durations less than half the mean passage time of RBCs. For vessel (1), the peak of the probability density is shifted towards longer void durations in the case of lingering with respect to non-lingering events. However, vessel (2) shows opposite behavior, which we conjecture to be a result of highly heterogeneous RBC distributions entering this branch. We measure equal lingering frequencies, as well as similar mean flowrates in both branches, $q_i = Q_i/Q_{\mathrm{M}} = \{0.55, 0.45\}$. The vessel diameters yield $d_i = \{4.6, 3.4\}\,\mu\mathrm{m}$.

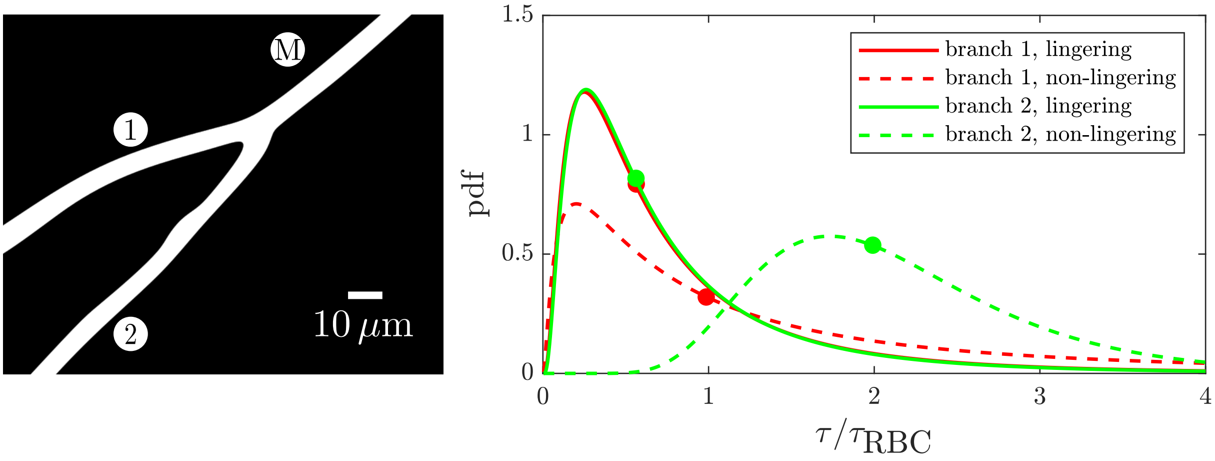


Figure 10: (left) Binary mask (evaluated manually), created according to the geometry in vivo. The flow is coming from the upper right corner (M) and exits in the two daughter branches (1) and (2), resp. as denoted in the scheme. Respective median values are marked by filled circles.

## S1.11 Geometry 11

For the geometry depicted in Fig. 11 we calculate the lingering frequencies as $n_{i,\text{linger}} = \{0.44, 0.37\}$, with $i \in \{1, 2\}$ referring to the vessel identifier. The calculated probabilities yield $P_i\left(\tau_{\text{void}} < 0.5\,\tau_{\text{RBC}}\right) = \{0.21, 0.44\}$ and $\tilde{P}_i\left(\tau_{\text{void}} < 0.5\,\tau_{\text{RBC}}\right) = \{0.03, 0.19\}$, resp. to find void durations less than half the mean passage time of RBCs. Also, the median void duration is increased in the case of lingering events with respect to non-lingering events. We again find the vessel with the higher mean flowrate obeying a higher lingering frequency compared to the adjacent vessel, since $q_i = Q_i/Q_{\text{M}} = \{0.52, 0.48\}$. The vessel diameters yield $d_i = \{3.6, 2.8\}\,\mu$m.

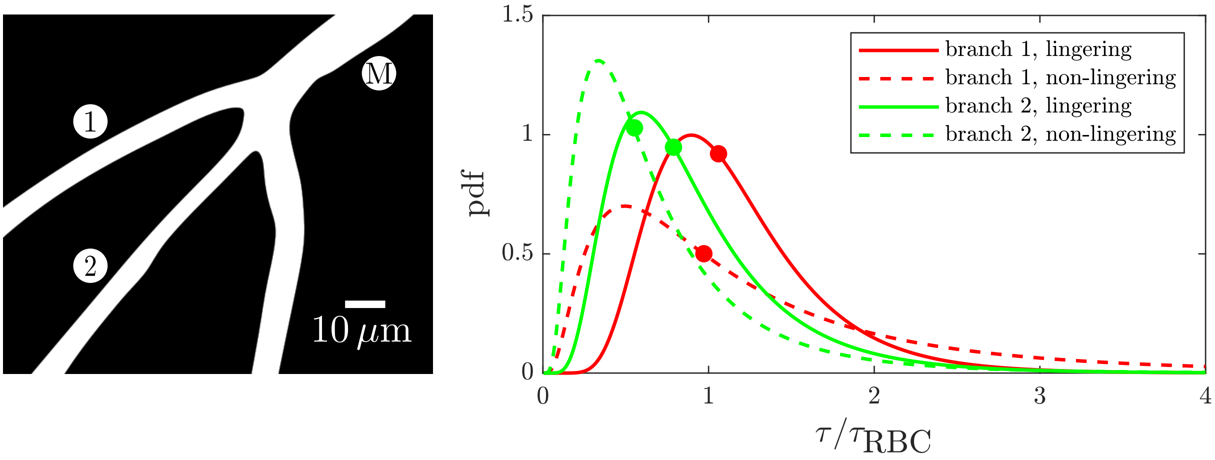


Figure 11: (left) Binary mask (evaluated manually), created according to the geometry in vivo. The flow is coming from the upper right corner (M) and exits in the three daughter branches. However, due to image quality, only vessels (1) and (2), resp. are suited for analysis. Respective median values are marked by filled circles.

## S1.12 Geometry 12

For the geometry depicted in Fig. 12 we calculate the lingering frequencies as $n_{i,\text{linger}} = \{0.11, 0.11\}$, with $i \in \{1, 2\}$ referring to the vessel identifier. The calculated probabilities yield $P_i\left(\tau_{\text{void}} < 0.5\,\tau_{\text{RBC}}\right) = \{0.17, 0.14\}$ and $\tilde{P}_i\left(\tau_{\text{void}} < 0.5\,\tau_{\text{RBC}}\right) = \{0.04, 0.02\}$, resp. to find void

durations less than half the mean passage time of RBCs. Also, the median void duration is increased in the case of lingering events with respect to non-lingering events. The mean flowrates in both branches are fairly similar, $q_i = Q_i/Q_\mathrm{M} = \{0.55, 0.45\}$, and again we measure equal lingering frequencies. Vessel diameters are measured as $d_i = \{2.9, 2.3\}\,\mu$m.

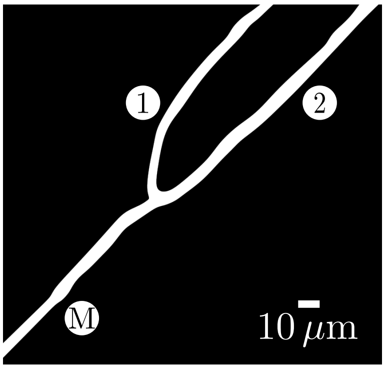


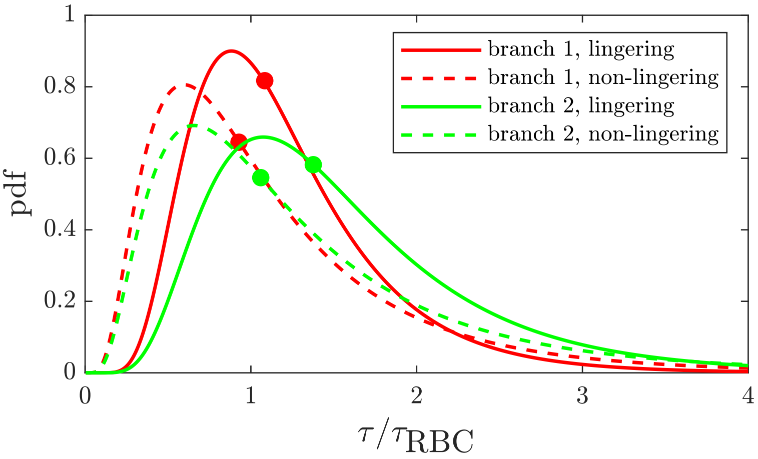


Figure 12: (left) Binary mask (evaluated manually), created according to the geometry in vivo. The flow is coming from the lower left corner (M) and exits in the two daughter branches (1) and (2), resp. as denoted in the scheme. Respective median values are marked by filled circles.

### S1.13 Geometry 13

For the geometry depicted in Fig. 13 we calculate the lingering frequency as $n_\text{1,linger} = \{0.04\}$. The calculated probabilities yield $P_1\left(\tau_\text{void} < 0.5\,\tau_\text{RBC}\right) = 0.35$ and $\tilde{P}_1\left(\tau_\text{void} < 0.5\,\tau_\text{RBC}\right) = 0.01$, resp. to find void durations less than half the mean passage time of RBCs. Also, the median void duration is increased in the case of lingering events with respect to non-lingering events. Due to experimantal restrictions, only vessel (1) can be analyzed properly. The diameter of this vessel is measured to be $d_1 = 2.7\,\mu$m.

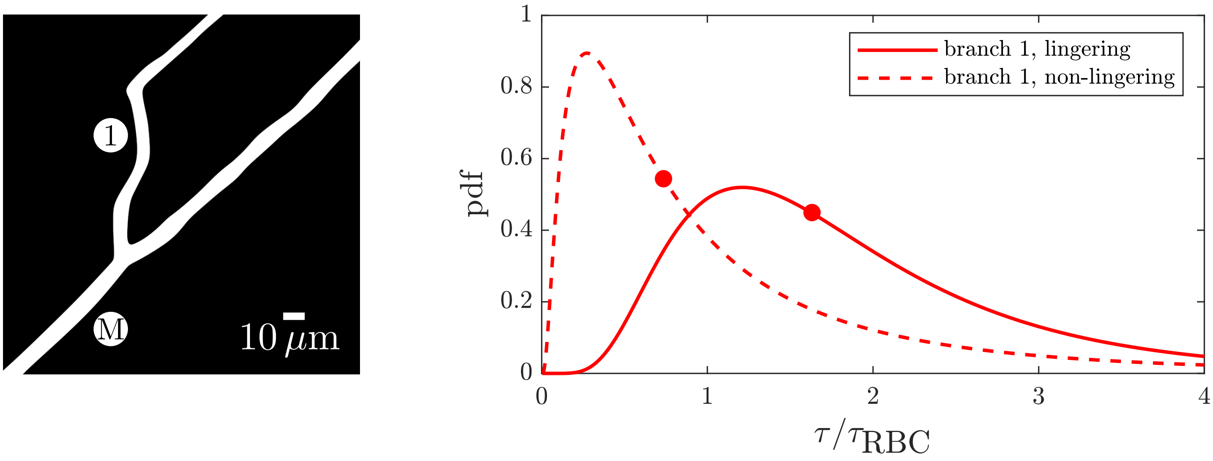


Figure 13: (left) Binary mask (evaluated manually), according to the geometry in vivo. The flow is coming from mother vessel (M) and exits in the two daughter branches. However, due to the focal plane, only vessel (1) is suitable for detecting RBCs. (right) Normalized void durations associated to non-lingering events in vessel (1) (dashed line) and for lingering events (solid line). In both cases, the normalization has been obtained by the mean of all passing RBCs in the respective branch, yielding a normalization by the flowrate. Respective median values are marked by filled circles.

### S1.14 Geometry 14

Of all RBCs observed flowing in the case of the geometry depicted in Fig. 14, only 2 showed lingering behavior. Thus the fraction of lingering cells is within the given accuracy vanishing, $n_{1,\mathrm{linger}} = \{0.00\}$, and we also do not show the probability density distribution of two single voids. However, for the sake of completeness we provide the probability densities of voids caused by all non-lingering events. $P_i\left(\tau_{\mathrm{void}} < 0.5\,\tau_{\mathrm{RBC}}\right) = 0.04$ and the vessel diameter is given as $d_1 = 3.4\,\mu$m.

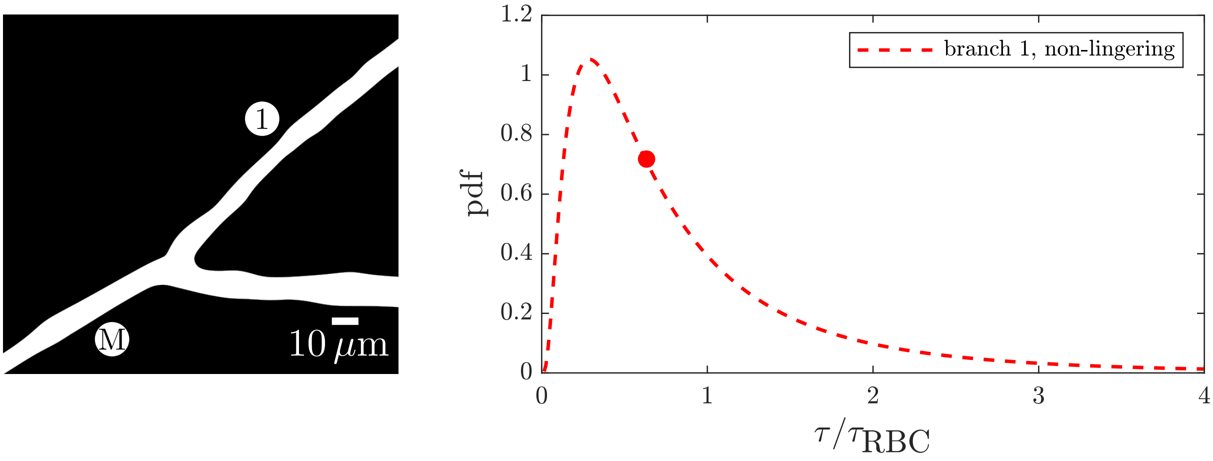


Figure 14: (left) Binary mask (evaluated manually), created according to the geometry in vivo. The flow is coming from the lower left corner (M) and exits in the two daughter branches. Due to image quality, only vessel (1) is suited for analysis. Respective median values are marked by filled circles.

## S2 Movie caption

Temporal evolution of microhematocrit evaluated in the red rectangle. The underlying geometry is identical to the one in Fig. 2 in the main manuscript. The highly heterogeneous behavior of the hematocrit value is contrasting the constant hematocrit value found in big vessels, such as e.g. arteries and originates from the particulate nature of blood and resulting heterogeneous distributions of RBCs within the microvascular system.

## S3 Movie caption

Intensity signal for the geometry discussed in the main manuscript (cf. Fig. 2 therein). The graph corresponds to the measured cumulative intensity along a perpendicular line segment with respect to the centerline of this branch, indicated by the red line segment in the top part. Values above the mean value can be regarded as voids, i.e. an absence of cells, whereas values below the mean value correspond to passing cells.

## S4 Movie caption

Two tracked RBCs with marked centroid positions and circumscribing ellipses. Whereas the RBC marked in red does not exhibit velocities below $v_{\text{RBC}} < 30\mu\text{m/s}$ at any time and therefore is not considered to show lingering behavior, the cell marked in green does obey velocities below the lingering velocity. Further, the circular region around the bifurcation apex is marked by a red dashed line, in which the velocity has to be less than $v_{\text{RBC}}$ for being associated with a lingering event. The red dashed line in the graph denotes the value of $v_{\text{RBC}}$. For the sake of visibility, we only analyze two RBCs.

## S5 Movie caption

According to the geometry depicted in Fig. 7 in the main manuscript we provide a video sequence showing the dynamics of RBCs approaching a bifurcation apex and distancing a confluence apex, resp. Centroid positions of individually flowing RBCs are tracked and marked with dots. In addition, the circumscribing ellipse is shown and the respective eccentricities as a function of centroid position. The playback speed of the video is set to be ($\times$ 0.1) real-time.
